# Supplementary material for: Collaborative Evolving Strategy for Automatic Data-Centric Development
Source: arXiv:2407.18690 source file (2024-07-26)
Supplement: Supplementary file 1 [file Scheduling_Agent_Prompt_and_Response.pdf]

## Scheduling Agent Prompt

{ User is trying to implement some factors in quant investment using Python code, You are an assistant who helps the user select the easiest-to-implement factors and some factors may be difficult to implement due to a lack of information or excessive complexity..

The user will provide the number of factor you should pick and information about the factors, including their descriptions, formulas, and variable explanations.

At the same time, user will provide with your former attempt to implement the factor and the feedback to the implementation. You need to carefully review your previous attempts. Some factors have been repeatedly tried without success. You should consider discarding these factors.

Here is the source data that user will use to implement the factors:{{ data\_info }}

Maybe some factors are dependent on other factors, that is, the function of some factors are contained in other factors, implement these factors first may help some other factors to implement. For instance, if acquiring the knowledge to complete task A could assist in completing task B, and task A is simpler than task B, we then establish a directed edge from A to B.

After recognizing the dependencies between different factors, you should consider to select those fundamental factors firstly. Please analyze the difficulties of the each factors and provide the reason and response the indices of selected implementable factor in the json format. Here is an example structure for the JSON output:

```
{
  "Dependency": "Dependency of different factors, you should response the dependencies in mermaid grammar with Annotation"
  "Analysis": "Analyze the difficulties of the each factors and provide the reason why the factor can be implemented or not."
  "selected_factor": "The indices of selected factor index in the list, like [0, 2, 3].The length should be the number of factor left after filtering."
}
```

## Scheduling Agent Response

{"Dependency":

graph TD

PB\_ROE --> PB\_ROE\_2

PB\_ROE --> PB\_ROE\_3

PB\_ROE --> PB\_ROE\_movement

PB\_ROE --> PB\_ROE\_movement\_10

PB\_ROE --> PB\_ROE\_movement\_20

ROE\_t --> ROE\_movement

ROE\_t --> ROE\_movement\_10

ROE\_t --> ROE\_movement\_20"

"Analysis": "Factors 0, 1, and 2 (PB\_ROE, PB\_ROE\_2, and PB\_ROE\_3) are variations of the same underlying concept, differing only in the division of the PB rank by a constant (1, 2, and 3 respectively), thus making implementation straightforward as they rely on the same inputs. Factor 9 (mid\_price) requires high-frequency data and involves calculations of standard deviation and mean of mid-prices, which are simple statistical operations on price data readily available. Factors 3, 4, and 5 (ROE\_movement\_10, ROE\_movement\_20, and ROE\_movement) require identifying the movement of ROE over different time windows which can be more complex due to the need to correctly handle time series data but are still feasible. Factors 6, 7, and 8 (PB\_ROE\_movement, PB\_ROE\_movement\_10, and PB\_ROE\_movement\_20) are dependent on both the calculation of PB\_ROE and the respective movement indicators for different time windows, making them more complex due to their dependency on the successful implementation of both PB\_ROE and the ROE movement indicators."

"selected\_factor": [0, 1, 9]}'
